# Supplementary material for: Ab-Initio Molecular Dynamics with Screened Lorentz Forces. Part I. Calculation and Atomic Charge Interpretation of Berry Curvature
Source: arXiv:2104.14861 source file (2021-04-30)
Supplement: Supplementary file 1 [file suppl_mat.pdf]

# Calculation of the Berry Curvature from Finite Difference for Molecular Systems

Tanner Culpitt,<sup>1</sup> Laurens D. M. Peters,<sup>1</sup> Erik I. Tellgren,<sup>1, a)</sup> and Trygve Helgaker<sup>1</sup>

*Hylleraas Centre for Quantum Molecular Sciences, Department of Chemistry,  
University of Oslo, P.O. Box 1033 Blindern, N-0315 Oslo,  
Norway*

(Dated: 28 April 2021)

---

<sup>a)</sup>Electronic mail: erik.tellgren@kjemi.uio.no

## I. CC-PVTZ+

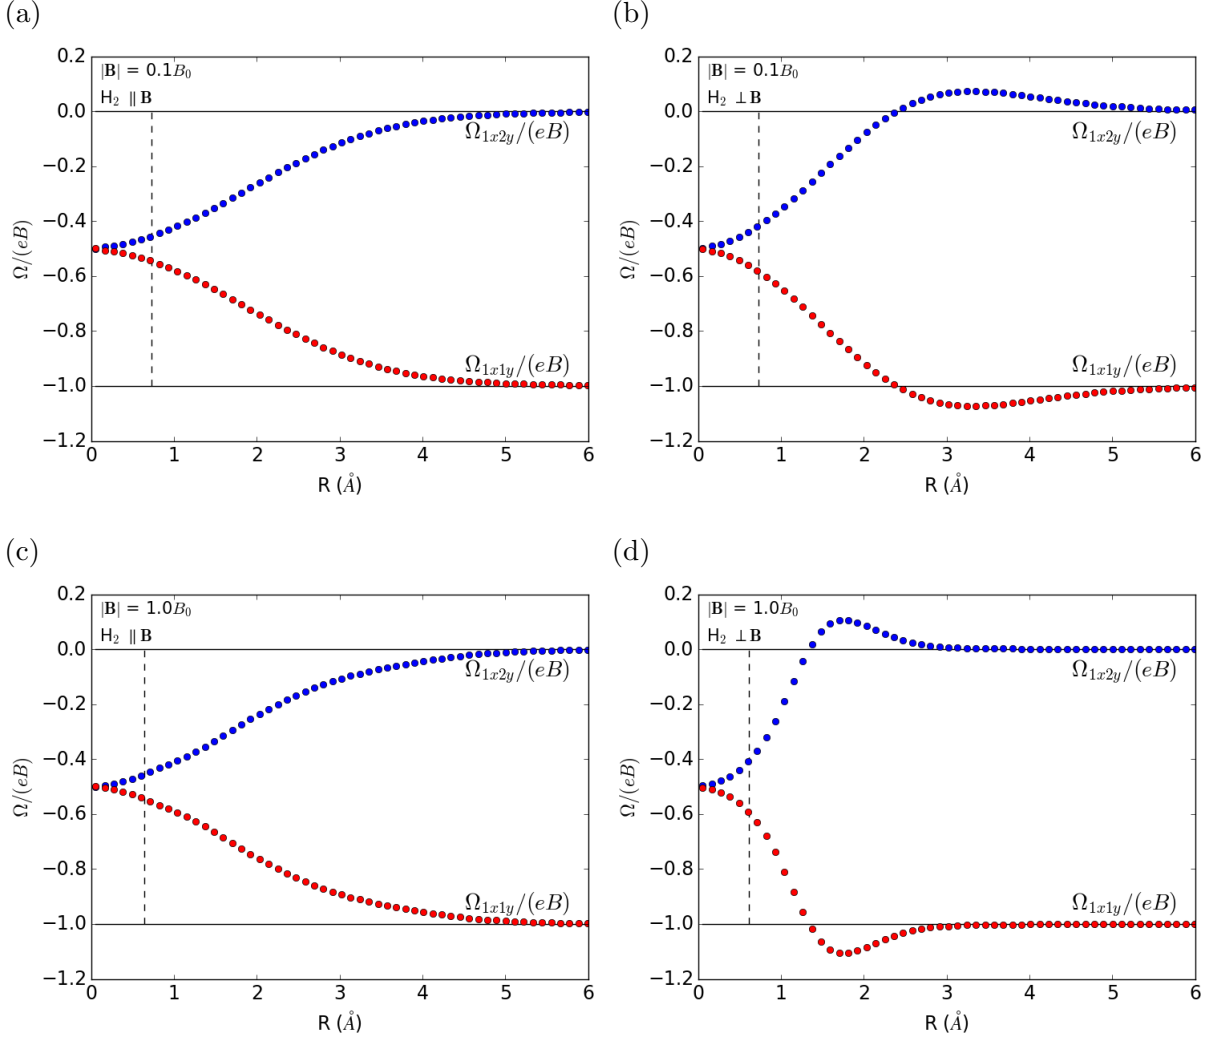

FIG. 1. Berry curvature of  $H_2$  for the RHF singlet state with the cc-pVTZ+ basis set for orientations parallel (a & c) and perpendicular (b & d) to the magnetic field. The field is oriented along the z-axis with a strength of  $|\mathbf{B}| = 0.1$  a.u. (a & b) and  $|\mathbf{B}| = 1.0$  a.u. (c & d). Molecular orientation perpendicular to the field is along the x-axis. The cc-pVTZ+ basis is comprised of cc-pVTZ hydrogen basis functions centered at the nuclei and a cc-pVDZ Helium ghost center placed at the center of mass. Equilibrium bond distances are 0.732 Å (a), 0.731 Å (b), 0.644 Å (c), and 0.612 Å (d) as shown by the vertical dashed lines in each plot.

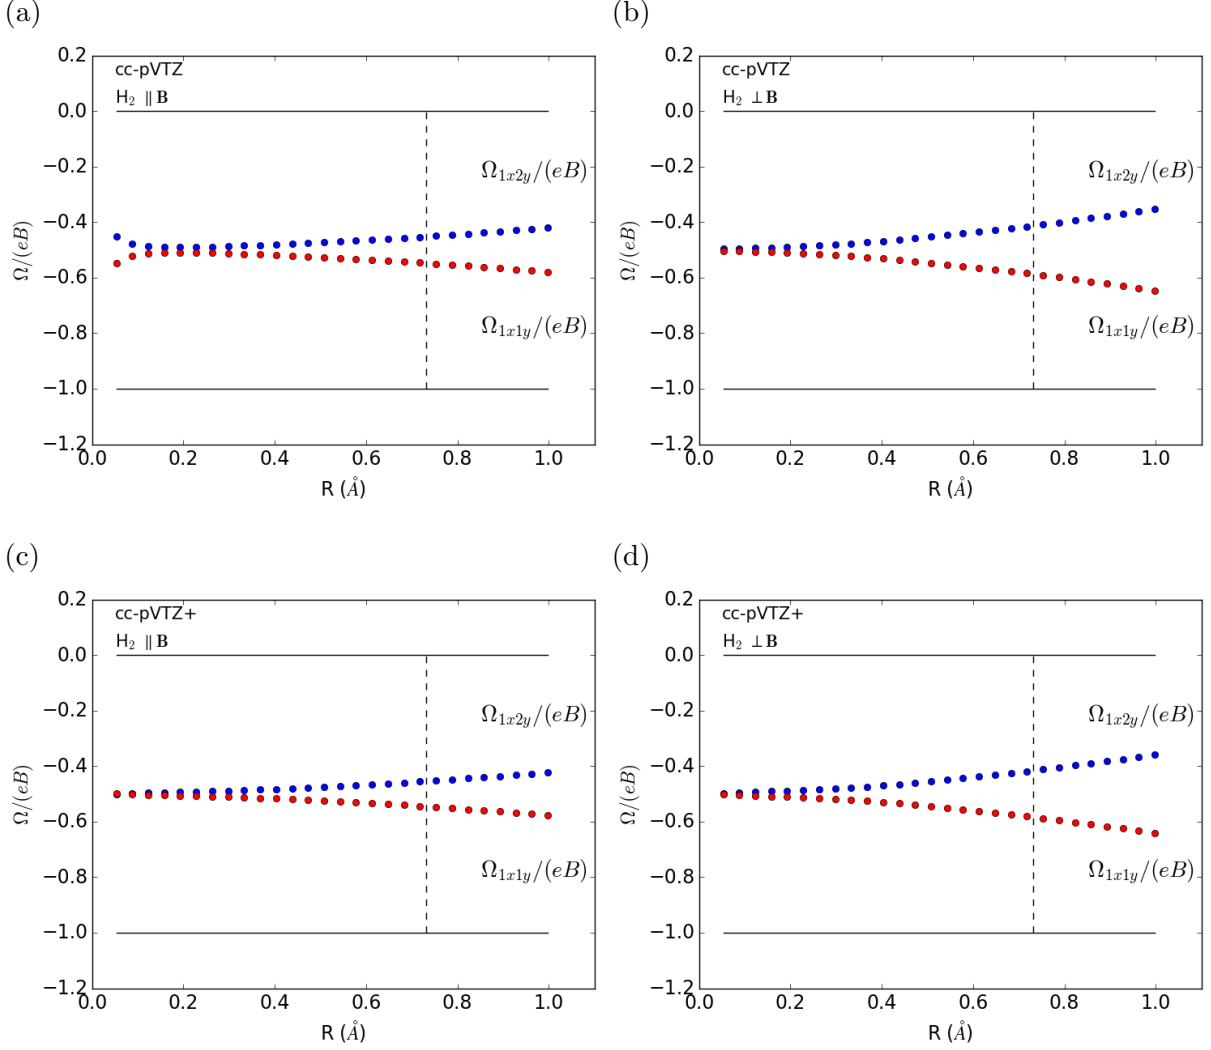

FIG. 2. Berry curvature of  $H_2$  for the RHF singlet state with the H cc-pVTZ basis set (a & b) and the cc-pVTZ+ basis set (c & d) for orientations parallel (a & c) and perpendicular (b & d) to the magnetic field. The field is oriented along the z-axis with a strength of  $|\mathbf{B}| = 0.1$  a.u. for all panels. The cc-pVTZ+ basis is comprised of cc-pVTZ hydrogen basis functions centered at the nuclei and a cc-pVDZ Helium ghost center placed at the center of mass. Molecular orientation perpendicular to the field is along the x-axis. Equilibrium bond distances are 0.732  $\text{\AA}$  (a & c), and 0.731  $\text{\AA}$  (b & d) as shown by the vertical dashed lines in each plot.
